# Supplementary material for: An Investigation of Warning Erroneous Chat Translations in Cross-lingual Communication
Source: arXiv:2408.15543 source file (2024-11-05)
Supplement: Supplementary file 1 [file appendix.tex]

\section{Crowdsourcing Information}
\label{appendix:A}
%\subsection{Instructions}
Below is the full description we presented to those who participated in our survey.

\paragraph{Instructions of the task}
This survey aims to investigate the effectiveness of the chat software's automatic translation system and its features when chatting with foreigners.

In the survey, your partner will speak to you in a language other than your native language. 
The translation system will translate your partner's messages into your language, and the chat will only be presented in your language. 
Your message will be translated into your partner's language, likewise.

Please read the chat log and choose one of the three options that you think is the most reasonable. 
The message sent to you will be displayed on the odd-numbered lines, and your answer will be displayed on the even-numbered lines.

After finishing the chat, please answer the related questions.
If you have any questions or comments, please fill in the feedback slots.

Your responses will be used for non-commercial academic research and recorded anonymously.
Please be careful not to include any personal information in the feedback, as we may consider them invalid.
Thank you for your cooperation.

\paragraph{Instructions of the rounds}

Please read the chat logs and choose the response you think is most reasonable from the three options.

Messages sent by your partner are displayed in odd-numbered lines, and your responses are displayed in even-numbered lines.
Please note that your partner is a non-native Chinese/Japanese speaker, and her/his messages are translated by the automatic translation function of the chat software.
Likewise, your message will be translated into her/his language before it is sent.

If you send a message that is translated incorrectly when you send it to the other person, you will see a warning message.
You can refer to this message to help you make your choice.\footnote{This instruction will only be shown to the participants in the round with the warning messages.}

%\section{Results of the Survey}
%\label{appendix:B}
%\input{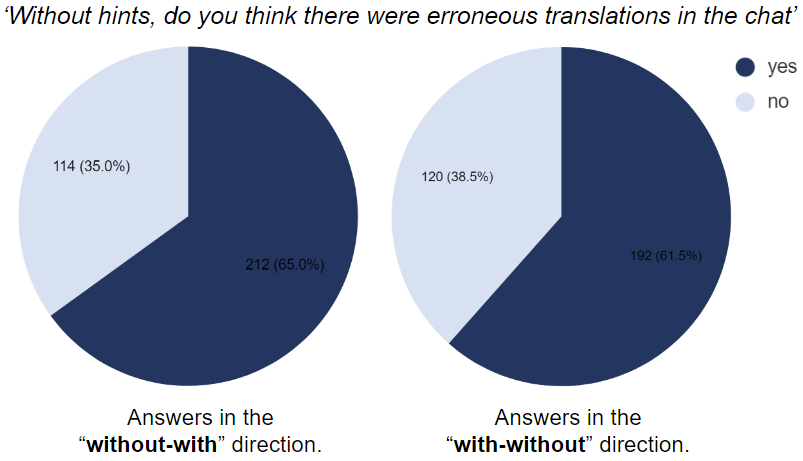}
%The results of how participants think the warning messages helped them continue the chat in the secondary survey.
